# Supplementary material for: Interlayer-Catalyst Method for Metal-Assisted Chemical Etching of Ultra-High Aspect Ratio Silicon Nanostructures
Source: arXiv:2602.10860 source file (2026-11-10)
Supplement: Supplementary file 1 [file Supporting_information.pdf]

Supporting information

# Interlayer-mediated catalyst engineering for ultra-high aspect ratio silicon nanostructures

*Bryan Peter Jost Benz*, Marco Stampanoni, Lucia Romano*

## Contents

Table SI 1: Cross-sectional SEM of commonly used resist showing the reflow problem during Pt deposition

Figure SI 1: Top-down and cross-sectional SEM of MacEtch experiment with conventional lift-off and Ar milling

Figure SI 2: Cross-sectional SEM of a pinned catalyst, here through alloying

Figure SI 3: Cross-sectional SEM of an $Cr/Al_2O_3$ interlayer with an undercut created by plasma etching

Figure SI 4: Cross-sectional SEM of the 1 cm x 1 cm patterned sample (second sample in Figure 6)

All standard resists show serious issues with reflowing.

Standard lift-off processes were attempted with different options for resists. These include the widely used PMMA and MMA as well as CSAR 62 which has been reported to perform better for Pt. All these resists lost their profile after the Pt deposition. The Pt deposition is realized in electron beam assisted evaporator (Bak evaporator from Evatec). We attribute this to the thermal reflow during the deposition.

| Resist | After development | After Pt deposition |
|---|---|---|
| PMMA | 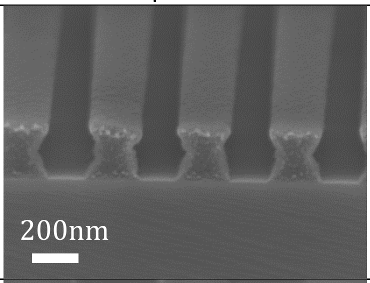 | 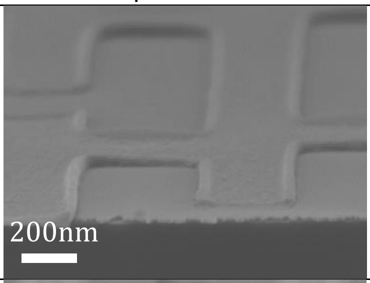 |
| MMA/PMMA bilayer | 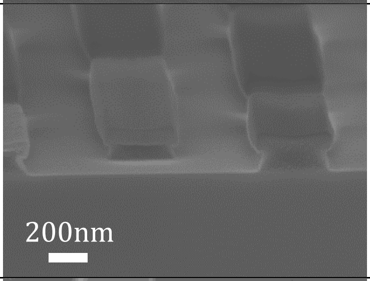 | 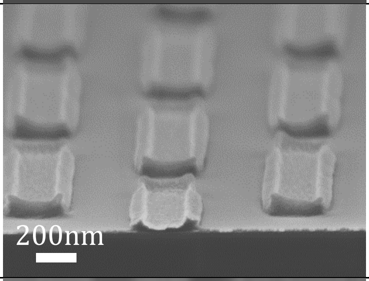 |
| CSAR 62 | 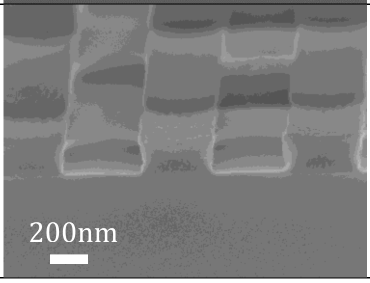 | 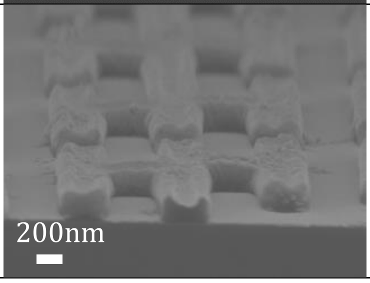 |

Table SI 1: Comparison of the stability of different resists for Pt deposition. The first column denotes the resist used to pattern the structure in EBL. The second column shows cross-sectional SEM of the patterned structures. The third column shows the result after depositing 12 nm of Pt on the sample. Clear deformation is visible in all three samples indicating that the resist is reflowing during Pt deposition. The overall yield and consistency of the lift-off process is low due to the severe deformation of the resist profile.

Conventional ways of patterning Pt directly show subpar MacEtch results

MacEtch standard patterning with lift-off and etching of the catalyst have been performed to limited experiments. The results show a lot of defects and poor pattern transfer even in the very early stages of the MacEtch process. In contrast, the interlayer approach has a much larger process window.

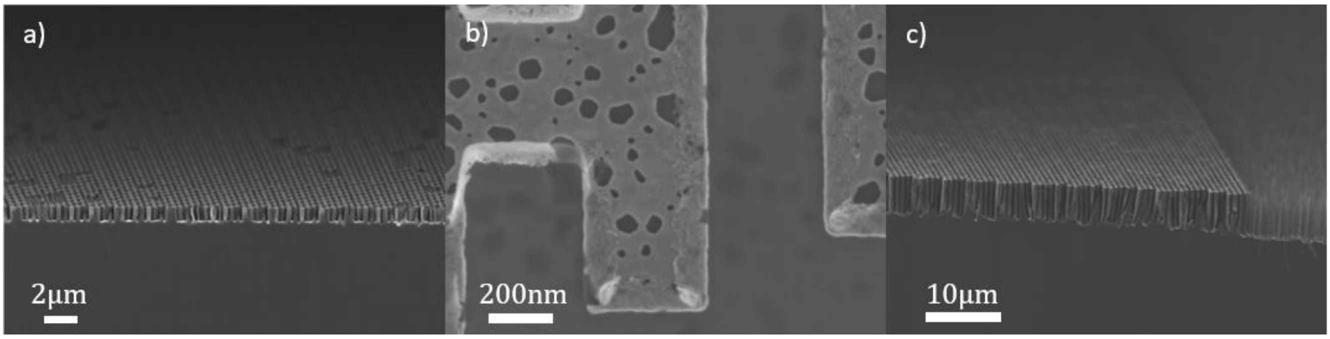


Figure Si 1: MacEtch using different, more classical, patterning methods. a) cross-sectional SEM of a sample created by lift-off with CSAR resist. Clearly visible are defects from poor lift-off on the top. In addition, there is no straight path of etching even at modest aspect ratio. b) and c) report attempts of Pt direct etching: the catalyst was first deposited on the silicon surface and then removed by Ar sputtering with a resist hard mask. Clearly visible in the top down SEM b) there are the fences arising from redeposition. After MacEtch in c) there is no straight etching, we observe local pinning and high porosity from isolated catalyst motion.

Pinning of the catalyst leads to porosity and removal of the catalyst without subsequent sinking of the catalyst

A central aspect of MacEtch is the mass transport of reactants and byproducts.[1], [2], [3], [4], [5] In particular, to remove the Si underneath the thin catalyst film, HF must reach it. The edges of the catalyst pattern provide preferential sites for the HF vapor to easily access the catalyst underneath, constituting faster etching sites that can eventually deform the pattern structure. The relevance of HF mass flow through the catalyst pattern has been demonstrated in previous work by introducing a dewetting process to create a random network of pores in the catalyst layer.[6] Dewetting of the metal catalyst on an oxygen-terminated silicon surface is caused by thermal treatment prior to etching. This causes the catalyst to form pores and cracks at the nanoscale.[7] The extra pores facilitate the penetration of HF through the catalyst, favoring uniform etching. Decreasing the size of the patterned features in the catalyst layer should progressively favor HF diffusion.

Chromium creates an alloy with Pt at elevated temperatures,[8] which conflicts with the temperature required for dewetting. Because Cr is a blocking material for MacEtch, a sample thermally treated at 250 °C with a Cr interlayer does not preserve the pattern transfer during MacEtch, and the etched structures present extended random porosity up to a few 100s nm below the catalyst. If a thermal treatment is required, Cr needs to be removed prior to dewetting.

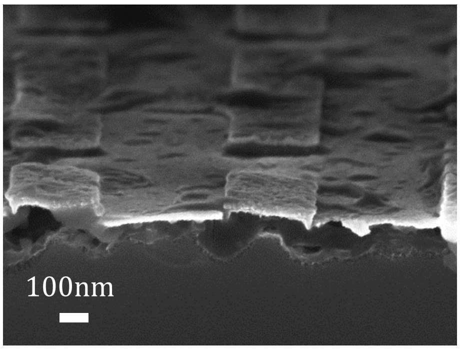


Figure SI 2: A cross-sectional view of a sample dewetted at 450°C without the removal of Cr before dewetting. The result is a large area of pinned catalyst and removal of the Si beneath the catalyst without a clear movement of the catalyst layer inside the silicon substrate typical of MacEtch.

Further option for creating artificial undercut with advanced patterning option

The Cr/$Al_2O_3$ interlayer can be processed with a liquid etchant or Cl2/O2 plasma for lateral thinning the Cr layer.

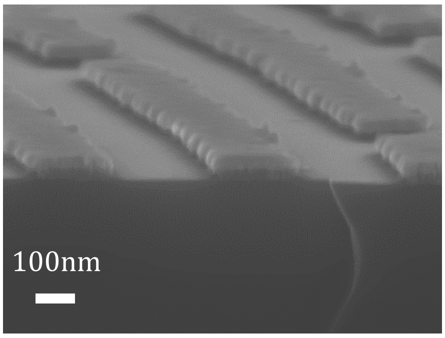


Figure SI 3: SEM in cross section of Cr/Al2O3 interlayer with artificial undercut created by plasma etching. The lower layer (Cr) is laterally etched, using the upper ($Al_2O_3$) as a hardmask.

Second run of a 1 cm x 1 cm sample etched with MacEtch shows worse pattern transfer, but no complete breaks

The sample of the second run in Figure 6 showed less pattern integrity, with multiple isolated breaks and non-straight etchings throughout the cross-section. Since a third attempt eight months later showed worse results and breaking, even with the dewetting treatment, we suspect an aging effect of the samples. This could be due to defects stemming from Cr alloying, worse Cr removal over time, or progressive environmental contamination diffusing beneath the catalyst, manifesting as degradation of the catalyst activity with age.

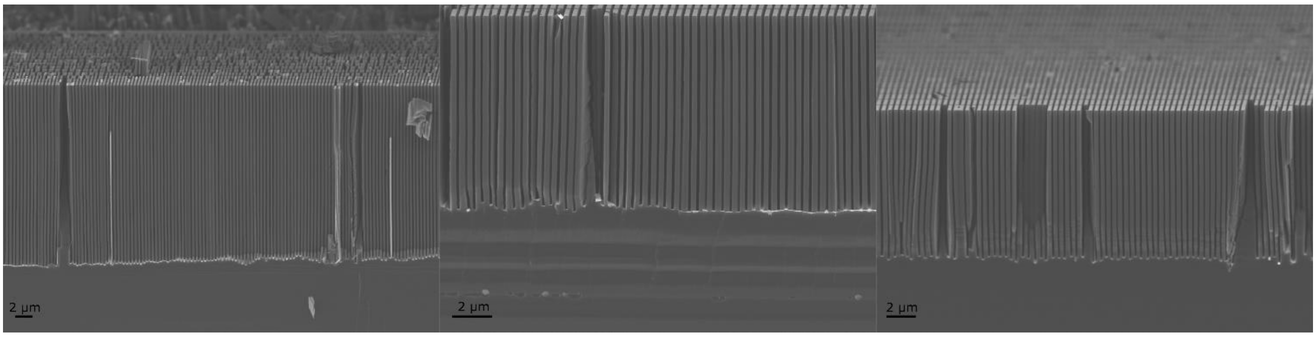


Figure SI 4: Cross-sectional SEM images of the second 1 cm x 1 cm sample etched in Figure 6. Local defects in the patterning decrease the quality compared to the first etched area reported in Figure 6.

[1] O.J. Hildreth, D.R. Schmidt, Vapor Phase Metal-Assisted Chemical Etching of Silicon, Advanced Functional Materials 24(24) (2014) 3827-3833.
[2] U. Han-Don, K. Namwoo, L. Kangmin, H. Inchan, H.S. Ji, Y. Young J., D. Peter, W. Munib, S. Kwanyong, Versatile control of metal-assisted chemical etching for vertical silicon microwire arrays and their photovoltaic applications, Scientific Reports 5 (2015) 11277.
[3] T.K. Kim, J.-H. Bae, J. Kim, Y.-C. Kim, S. Jin, D.W. Chun, Bulk Micromachining of Si by Annealing-Driven Magnetically Guided Metal-Assisted Chemical Etching, ACS Applied Electronic Materials 2(1) (2020) 260-267.
[4] Z. Huang, N. Geyer, P. Werner, J. de Boor, U. Gösele, Metal-Assisted Chemical Etching of Silicon: A Review, Advanced Materials 23(2) (2011) 285-308.
[5] N. Geyer, B. Fuhrmann, Z. Huang, J. de Boor, H.S. Leipner, P. Werner, Model for the Mass Transport during Metal-Assisted Chemical Etching with Contiguous Metal Films As Catalysts, The Journal of Physical Chemistry C 116(24) (2012) 13446-13451.
[6] L. Romano, J. Vila-Comamala, K. Jefimovs, M. Stampanoni, High-Aspect-Ratio Grating Microfabrication by Platinum-Assisted Chemical Etching and Gold Electroplating, Advanced Engineering Materials 22(10) (2020) 2000258.
[7] C.V. Thompson, Solid-State Dewetting of Thin Films, Annual Review of Materials Research 42(1) (2012) 399-434.
[8] M. Seifert, E. Brachmann, G. Rane, S. Menzel, T. Gemming, Capability Study of Ti, Cr, W, Ta and Pt as Seed Layers for Electrodeposited Platinum Films on γ-Al2O3 for High Temperature and Harsh Environment Applications, Materials 10(1) (2017) 54.
